# Supplementary material for: Scrutinizing Hall effect in Mn$_{1-x}$Fe$_{x}$Si: Fermi surface evolution and hidden quantum criticality
Source: arXiv:1507.05227 ancillary file (2015-07-18)
Supplement: Supplementary file 1 [file Supplement_Glushkov.pdf]

**Supplementary materials to the manuscript of V.V.Glushkov et al.**
**"Scrutinizing Hall effect in $Mn_{1-x}Fe_xSi$:**
**Fermi surface evolution and hidden quantum criticality"**

## Experimental details and experimental method

The temperature and field dependencies of Hall resistivity have been measured on the single crystals of $Mn_{1-x}Fe_xSi$ with Fe content $x$<0.3 in magnetic fields below 5T at temperatures 2-60 K. X-ray diffraction data confirmed the high quality of the crystals grown by Czochralsky technique. EPMA was applied to determine the real content of Fe and to check the deviation from the stoichiometric composition, which doesn't exceed $y\approx0.015$ in the $(Mn_{1-x}Fe_x)_{1+y}Si_{1-y}$ chemical formula. More detailed information on the structural and magnetic properties of the single crystals can be found in the previous reports [5,8,14]). The resistivity and Hall resistivity were measured in the same run by using the standard six-probe scheme and sweeping magnetic fields in two opposite directions at constant temperature. The demagnetization factors of the samples under investigation were estimated within standard approach [S1]. The magnetization data M(H,T) were measured by using MPMS-5 setup.

## Experimental data

The experimental data for Hall resistivity $\rho_H$(B,T) and magnetization M(B,T) are presented in Figs.S1-S2. The general trends in $\rho_H$ and M as well as their absolute values are in good agreement with the previously reported data [18]. The substitution of Mn by Fe in the P phase is found to change the sign of the Hall effect from positive one observed for pure MnSi (Fig.S1a, see also [16-19]) to the negative values detected in the compounds with Fe content $x$>0.1 (Fig.S1c-h). Besides, a complicated non-monotonous field dependence of the $\rho_H(B,T_0)$ isotherms is observed for the $x$=0.054 single crystal (see Fig.S1b and open squares in Fig.S3).

## Scaling analysis of Hall resistivity

Analysis of the $\rho_H(T,B_0)$ behavior on the scaling plots for two different approaches $n$=1 and $n$=2 shows that the best linearization of the data in the P-phase of $Mn_{1-x}Fe_xSi$ can be achieved when plotting the $\rho_H/B_0=f(\rho M/B_0)$ graph (Fig.S4). Indeed, the linear dependences of $\rho_H/B_0=R_H+S_1\cdot\mu_0\rho M/B_0$ shown by dotted lines in Fig.4 demonstrate nice correlation with experimental data. This observation means that AHE in the P-phase of $Mn_{1-x}Fe_xSi$ is controlled by extrinsic mechanism contributed from skew scattering of charge carriers as it was earlier shown for pure MnSi [19]. Separating between ordinary and anomalous contribution to Hall resistivity in the data of Fig.4 shows that Hall constant $R_H$ determined by the intersection of the best fits with y axis rises monotonously with increasing of Fe content from negative ($x$<0.11) to positive ($x$>0.11) values. In contrary, the AHE constant $S_1$, which defines the slope of the linear fits, decreases under Fe doping becoming negative for the $Mn_{1-x}Fe_xSi$ single crystal with the lowest available concentration of iron ($x$=0.054, Fig.S4). Besides, the universal linear fit of the $\rho_H/B_0=f(\rho M/B_0)$ data for each sample of $Mn_{1-x}Fe_xSi$ means that neither $R_H(x)$ nor $S_1(x)$ depend on temperature in the studied range of temperatures $T_S<T<60$ K.

The correctness of the aforementioned analysis is strongly supported by the field and temperature dependences of Hall resistivity. Indeed, comparing of the $\rho_H(B,T_0)$ and $\rho_H(T,B_0)$ data in Figs.2 and S3 with the curves calculated from the resistivity and magnetization in the $\rho_H^a\propto\rho M$ approximation (solid lines in Figs.2 and S3) show excellent agreement between experimental and simulated data. The deviation of the simulated curves from the experimental values of Hall resistivity detected for $x$=0.054 single crystals in magnetic field $B$>1T (Fig.S3) is believed to result from the field induced suppression of spin fluctuations, which should lead to the violation of the $\rho_H^a\propto\rho M$ asymptotic in moderate magnetic field similar to the case of pure MnSi [19]. At

the same time, the increase of Fe content expands the range of magnetic fields, in which the skew scattering of charge carriers defines the AHE in these compounds (Fig.S3).

## RKKY exchange for two groups of charge carriers

If quadratic and isotropic dispersion law is assumed for both electrons and holes, the corresponding Fermi energies are given by $E_{Fe,h}=\hbar^2 k_{Fe,h}/2m_{e,h}$ and Fermi momenta scales with concentration as $k_{Fe}(x)=[3\pi^2 n(x)]^{1/3}$ and $k_{Fh}(x)=[3\pi^2 p(x)]^{1/3}$. So exchange interaction $J(r)$ between LMMs at the distance $r$ in the presence of electrons and holes is the sum of contributions from electrons and holes [27]

$$J(r)=J_e(r)+J_h(r)=\frac{const}{r^4}\left[m_e\varphi(2k_{Fe}r)+m_h\varphi(2k_{Fh}r)\right], \qquad \text{(S1)}$$

where $\varphi(z)=z\cos(z)-\sin(z)$. In the framework of the assumptions made, the Equation (S1) can be transformed to the form of Eq.(3).

## References

S1. A. Aharoni, **Demagnetizing factors for rectangular ferromagnetic prisms**, J. Appl. Phys., **83**, 3432 (1998).

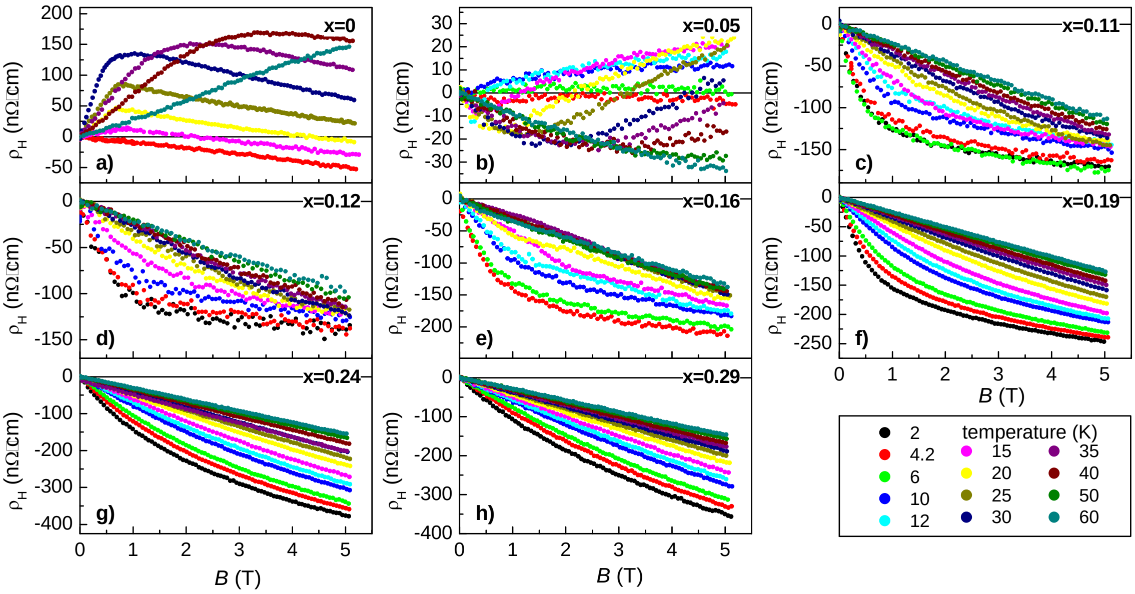


**Fig.S1** Temperature dependences of the Hall resistivity of $Mn_{1-x}Fe_xSi$. The numbers in the right top corner correspond to the concentration of iron.

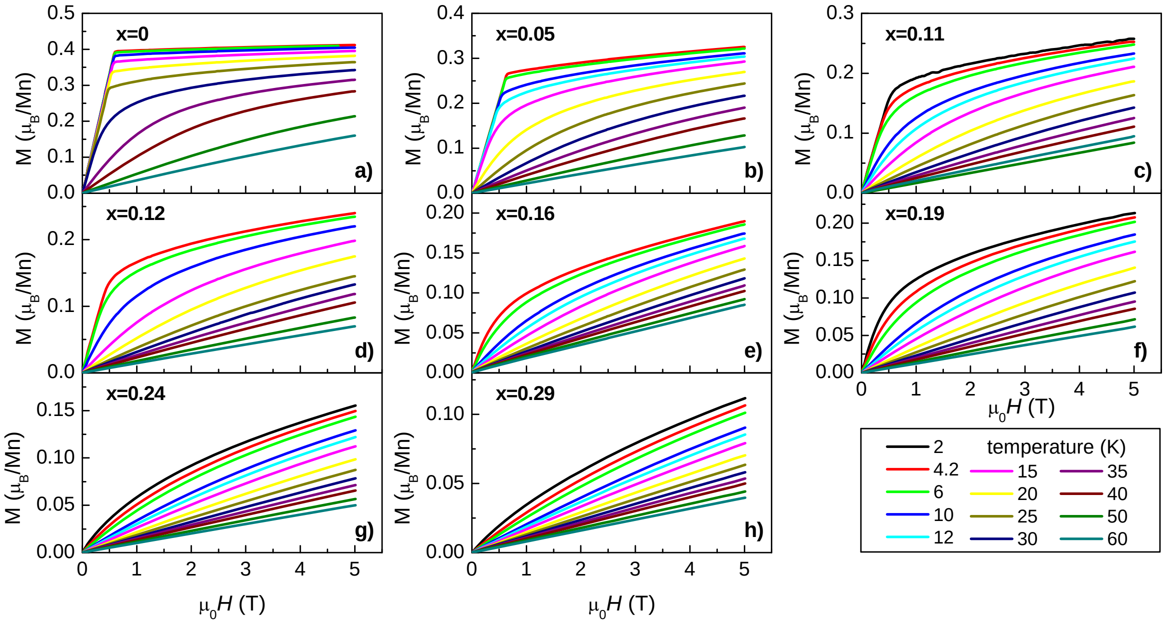


**Fig.S2** Temperature dependences of the magnetization of $Mn_{1-x}Fe_xSi$. The numbers in the left top corner correspond to the concentration of iron.

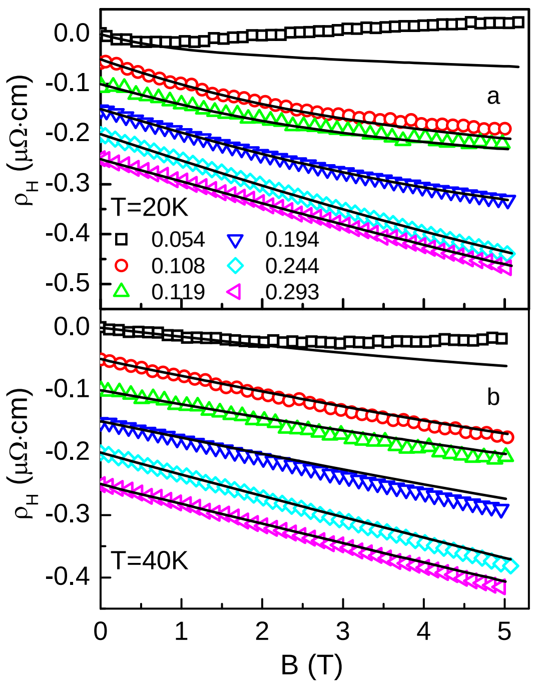


**Fig.S3** Isotherms of Hall resistivity $\rho_H$ as a function of magnetic induction *B* (symbols) in the P-phase of $Mn_{1-x}Fe_xSi$ solid solutions measured at (a) *T*=20 K and (b) *T*=40 K. Solid lines are the fits by $\rho_H = R_H B + \mu_0 S_1 \rho M$ with parameters $R_H$(x) and $S_1$(x) shown in Fig.5a. For clarity the data are shifted down by 50 nΩ·cm for each composition with the respective $\rho_H$=0 values shown by dashed lines.

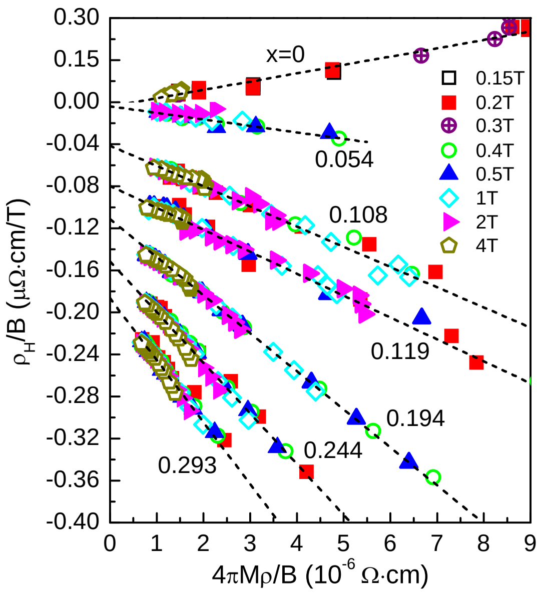


**Fig.S4.** Scaling plots of Hall resistivity $\rho_H/B_0=f(\mu_0 S_1 \rho M/B_0)$ in the P- phase of $Mn_{1-x}Fe_xSi$ solid solutions for selected magnetic fields shown in the legend. Solid lines are the best linear fits of the data. For clarity the data for $x>0.1$ are shifted down by 40 nΩ·cm/T for each composition. Note the different scale of y axis for positive and negative values.
